# Supplementary material for: Collision Detection Accelerated: An Optimization Perspective
Source: arXiv:2205.09663 source file (2022-05-20)
Supplement: Supplementary file 1 [file appendix.tex]

\appendix
\subsection{Hill-climbing}
\label{sec:appendix_hill_climbing}
A mesh containing~$N_v$ vertices is fully described by a list of vertices~$[\bm v_i]_{1 \leq N_v}$ and~$N_v$ lists of neighbor indices such that list~$i$ contains the indices of the neighbors of~$\bm v_i$.
In the following, we give ourselves a convex mesh~$\mathcal{A}$.
A support call in direction~$\bm d$ thus consists in finding a point~$\bm s$ among vertices~$[\bm v_i]$ which verifies:
%%%%%%%%%% EQUATION %%%%%%%%%% 
%%%%%%%%%%%%%%%%%%%%%%%%%%%%%%%
\begin{equation}
    \begin{aligned}
        \bm s \in \argmin_{i \in [1, N_v]} \langle \bm v_i, \bm d \rangle    
    \end{aligned}
\end{equation}
%%%%%%%%%%%%%%%%%%%%%%%%%%%%%%%
%%%%%%%%%%%%%%%%%%%%%%%%%%%%%%%
A naive support call algorithm for a convex mesh thus consists in computing all dot-products~$\langle \bm v_i , \bm d \rangle$ and using point~$\bm v_i$ with the lowest dot-product as a support point.
In order to reduce the amount of the support call on a convex mesh, we instead the use~\textit{hill-climbing} method.
Given a mesh and a starting index~$i_0$, the hill-climbing algorithm consists in starting on vertex~$\bm v_{i_0}$ of the mesh, computing the dot-product of vectors~$\bm v_i$ and its neighors with~$\bm d$.
Since the mesh is convex, if neigbor~$\bm v_j$ of~$\bm v_{i_0}$ has a lower dot-product with~$\bm d$ than~$\bm v_{i_0}$, we move to~$\bm v_j$ and repeat the operation.
Otherwise we stop and use the point we are at as a support point in direction~$\bm d$.
The hill-climbing algorithm is summed up in Alg.~\ref{alg:hill_climbing}.
Since the algorithm returns a vertex~$v_{i_0}$ as well as the index~$i_0$ associated to that vertex, we can use index~$i_0$ the next time we call a support operation on that same convex mesh.
%%%%%%%%%% ALGORITHM %%%%%%%%%% 
%%%%%%%%%%%%%%%%%%%%%%%%%%%%%%%
\begin{algorithm}[H]
  \caption{Hill-climbing algorithm}
  \begin{algorithmic}[1]
    \State \textbf{Let} $\bm d \in \Rthree,\, i_0 \in [1, N_v],\, V=[\bm v_i]_{1 \leq N_v}$
    \State $\text{stopped\_climbing} \gets \text{False}$
    \State $\bm v \gets V[i_0]$
    \State $r_{\min} \gets \langle \bm v, \bm d\rangle$
    \While{not stopped\_climbing}
        \State $\text{improved} \gets \text{False}$
        \State $L(v) \gets \text{list of indices of neighbors of } \bm v$
        \For{$i \in L(v)$}
            \State $r \gets \langle \bm{V[i]}, \bm d\rangle$
            \If{$r < r_{\min}$}
                \State $i_0 \gets i$
                \State $\text{improved} \gets \text{True}$
                \State $r_{\min} \gets r$ 
            \EndIf
        \EndFor
        \If{not improved}
            \State $\text{stopped\_climbing} \gets \text{True}$
        \EndIf
    \EndWhile
    \State \textbf{return } $V[i_0],\, i_0$
  \end{algorithmic}
  \label{alg:hill_climbing}
\end{algorithm}
%%%%%%%%%%%%%%%%%%%%%%%%%%%%%%%
%%%%%%%%%%%%%%%%%%%%%%%%%%%%%%%
